# Supplementary material for: Nonreciprocal pattern formation of conserved fields
Source: arXiv:2306.08868 source file (2024-04-22)

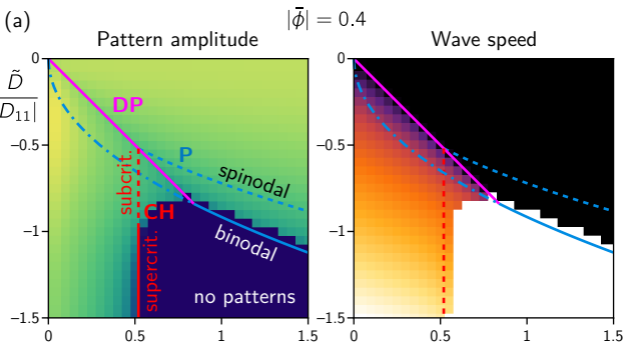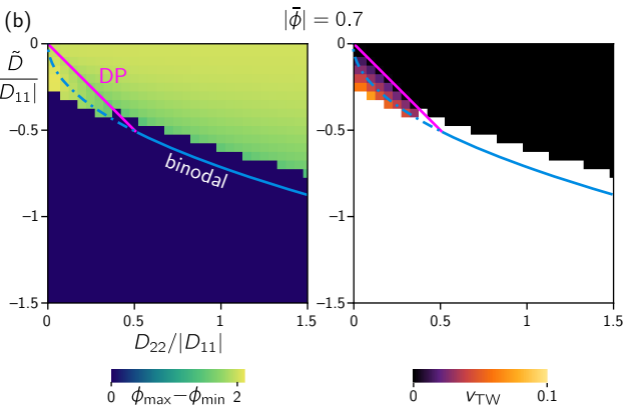



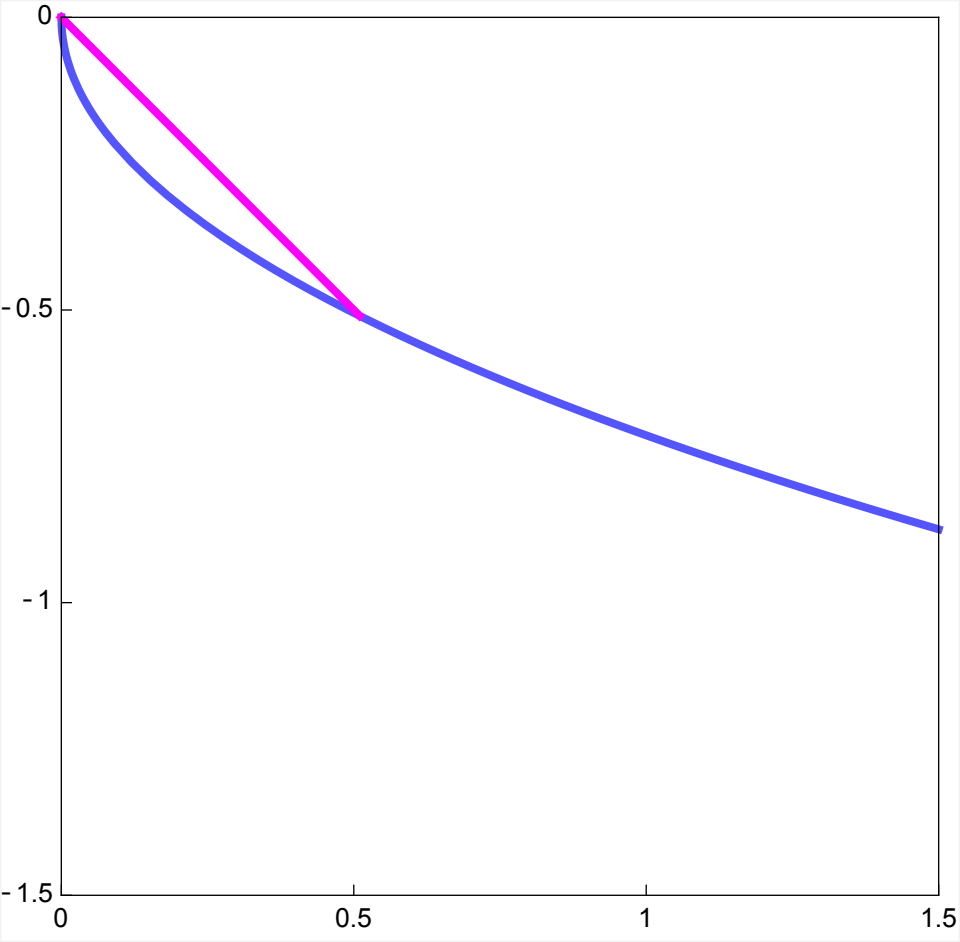

Supplement: Supplementary file 1 [file phase-diagrams_appendix.pdf]
